# Supplementary material for: The Multi-Trip Time-Dependent Mix Vehicle Routing Problem for Hybrid Autonomous Shared Delivery Location and Traditional Door-to-Door Delivery Modes
Source: arXiv:2503.05842 source file (2025-03-07)
Supplement: Supplementary file 1 [file Appendix.tex]

% Appendix.tex
\appendix

\section{Appendix}
This is the appendix section.
